# Supplementary material for: In-vehicle alertness monitoring for older adults
Source: arXiv:2208.08091 source file (2022-08-17)
Supplement: Supplementary file 1 [file appendix.tex]

\section{Appendix}
\label{appendix}
